# Supplementary material for: Providing Insights for Queries affected by Failures and Stragglers
Source: arXiv:2002.01531 source file (2020-02-04)
Supplement: Supplementary file 1 [file appendix.tex]

\section{Sampling Designs}
\label{apx:sampling}

\introparagraph{1-Stage Sampling.}

If the sampling size $n_S$ is fixed (e.g., for SRS without replacement), a computationally efficient formula for variance and an estimator for the variance is as follows:
\begin{align}
\Var(\hat{t}) = -\frac{1}{2}\sum_{i = 1}^{N} \sum_{j = 1}^{N} \Delta_{ij} (\frac{t_i}{\pi_i} - \frac{t_j}{\pi_j})^2 \\
\widehat{\Var}(\hat{t}) = -\frac{1}{2}\sum_{i \in S} \sum_{j \in S} \frac{\Delta_{ij} }{\pi_{ij}}(\frac{t_i}{\pi_i} - \frac{t_j}{\pi_j})^2 
\end{align}

\introparagraph{2-stage Sampling.}
We present here the formulas for 2-stage sampling as an example of the complete
calculation. In 2-stage sampling, for every $i \in C_I$, we choose a sample $S_i$ from cluster $C_i$.
The estimator for $c_i$ is then given by  
$$\hat{c}_{i} = \sum_{k \in S_{i}} \frac{t_k}{\pi_{k|i}}$$
where $\pi_{k|i}$ is the probability that tuple $k$ is chosen from the cluster $C_i$.
Hence, the HT estimator becomes:
\[
\hat{t} =  \sum_{i \in S_I} \frac{1}{\pi_{Ii}} \cdot \left(  \sum_{k \in S_{i}} \frac{t_k}{\pi_{k|i}} \right) 
\]

To compute the variance $V_i$ of cluster $C_i$ and its estimation $\hat{V}_i$, we first need the
inclusion probabilities:
\begin{align*}
  \pi_{kl} =
\begin{cases}
  \pi_{Ii}\pi_{k|i} & \text{ if } k = l \in C_i \\
 \pi_{Ii}\pi_{kl|i} & \text{ if } k \& l  \in C_i, k \neq l \\
  \pi_{Iij}\pi_{k|i} \pi_{l|j} & \text{ if } k \in C_i \text{ and }  l \in C_j (i \neq j)\\
\end{cases}
\end{align*} 

Then, the variance and unbiased estimator for the variance formulas for the second stage are given by:
\begin{align}
V_i = \sum_{k \in C_i} \sum_{l \in C_i} \Delta_{kl|i} \frac{t_k}{\pi_{k|i}} \frac{t_l}{\pi_{l|i}} \\
\hat{V}_i = \sum_{k \in S_i} \sum_{l \in S_i}  \frac{\Delta_{kl|i}}{\pi_{kl|i}}\frac{t_k}{\pi_{k|i}} \frac{t_l}{\pi_{l|i}}
\end{align}

The variance of the two stage sampling method is given by:

\begin{align*}
\Var(\hat{t}) = V_{stage_1}  + V_{stage_2}
=  \sum_{i \in C_I} \sum_{j \in C_I} \Delta_{Iij} \hat{c}_{i}\hat{c}_{j} + \sum_{C_I} \frac{V_i}{\pi_{Ii}}
\end{align*}  
and the variance estimator as:
\begin{align*}
\widehat{\Var}(\hat{t}) = \hat{V}_{stage_1}  + \hat{V}_{stage_2}
=  \sum_{i \in S_I} \sum_{j \in S_I} \hat{\Delta}_{Iij} \frac{\hat{c}_{i}}{\pi_{Ii}} \frac{\hat{c}_{j}}{\pi_{Ij}}
+ \sum_{S_I} \frac{\hat{V}_i}{\pi_{Ii}}
\end{align*}

In practice, computing the variances from the previous formulas is computationally inefficient.  To overcome this issue, we can reduce the previously given formulas to a more computationally efficient variance formula (for fixed-size sampling)~\cite{bookSarndal}.
